# Supplementary material for: Temporal Flow Matching for Learning Spatio-Temporal Trajectories in 4D Longitudinal Medical Imaging
Source: arXiv:2508.21580 source file (2025-08-29)
Supplement: Supplementary file 1 [file Appendix.tex]

\documentclass[../paper]{subfiles}
\begin{document}
\section{Experimental specifications}
\subsection{Model Specifications}

\subsection{Scaling ConvLSTM}

\end{document}
